# Supplementary material for: A Multi-Scale Approach to Simulate the Nonlinear Optical Response of Molecular Nanomaterials
Source: arXiv:2308.16625 ancillary file (2023-08-31)
Supplement: Supplementary file 1 [file SI.pdf]

# Supplement Information: A Multi-Scale Approach to Simulate the Nonlinear Optical Response of Molecular Nanomaterials

Benedikt Zerulla*,[1] Dominik Beutel,[2] Christof Holzer,[2] Ivan Fernandez-Corbaton,[1] Carsten Rockstuhl*,[1, 2] and Marjan Krstić*[2]

[1)] *Institute of Nanotechnology, Karlsruhe Institute of Technology (KIT), 76344 Eggenstein-Leopoldshafen, Germany*

[2)] *Institute of Theoretical Solid State Physics, Karlsruhe Institute of Technology (KIT), 76131 Karlsruhe, Germany*

(Dated: 31 August 2023)

## I. LINEAR T-MATRIX FORMALISM

In the main article, the Hyper-T-matrix is introduced, which relates the scattering coefficients at a higher-order frequency to multiple incident fundamental electric fields. For linear optical processes, the T-matrix formalism is used[1]. For better readability, we omit the frequency in the following as an argument. In the T-matrix formalism, one expands the electric field outside an isolated scatterer in the frequency domain as

$$\begin{aligned}\boldsymbol{E}(\boldsymbol{r}) = \sum_{l=1}^{\infty}\sum_{m=-l}^{l}\Big(& a_{lm,\mathrm{N}}\boldsymbol{N}_{lm}^{(1)}(k_\mathrm{h}\boldsymbol{r}) + a_{lm,\mathrm{M}}\boldsymbol{M}_{lm}^{(1)}(k_\mathrm{h}\boldsymbol{r}) \\ &+ c_{lm,\mathrm{N}}\boldsymbol{N}_{lm}^{(3)}(k_\mathrm{h}\boldsymbol{r}) + c_{lm,\mathrm{M}}\boldsymbol{M}_{lm}^{(3)}(k_\mathrm{h}\boldsymbol{r})\Big),\end{aligned} \tag{1}$$

with $\boldsymbol{N}_{lm}^{(1)}(k_\mathrm{h}\boldsymbol{r})$ and $\boldsymbol{M}_{lm}^{(1)}(k_\mathrm{h}\boldsymbol{r})$ being incident and $\boldsymbol{N}_{lm}^{(3)}(k_\mathrm{h}\boldsymbol{r})$ and $\boldsymbol{M}_{lm}^{(3)}(k_\mathrm{h}\boldsymbol{r})$ being scattered vector spherical waves. $\boldsymbol{N}$ are transverse magnetic (TM) and $\boldsymbol{M}$ are transverse electric (TE) modes in the case of regular waves[2,3]. Constructing two column vectors which consist of the expansion coefficients $a_{lm}$ and $c_{lm}$, one can relate them with the T-matrix,

$$\boldsymbol{c} = \mathbf{T}\boldsymbol{a}. \tag{2}$$

Using Equation (6) from[2], the dipolar ($l = 1$) T-matrix of a molecular unit cell can be computed from its dipolar polarizability tensors,

$$\begin{aligned}\begin{pmatrix}\mathbf{T}_\mathrm{NN} & \mathbf{T}_\mathrm{NM} \\ \mathbf{T}_\mathrm{MN} & \mathbf{T}_\mathrm{MM}\end{pmatrix} = & \frac{\mathrm{i}c_\mathrm{h}Z_\mathrm{h}k_\mathrm{h}^3}{6\pi} \\ & \begin{pmatrix}\mathbf{C}\left(\boldsymbol{\alpha}_\mathrm{ee}\right)\mathbf{C}^{-1} & \mathbf{C}\left(-\mathrm{i}\boldsymbol{\alpha}_\mathrm{em}/Z_\mathrm{h}\right)\mathbf{C}^{-1} \\ \mathbf{C}\left(\mathrm{i}\boldsymbol{\alpha}_\mathrm{me}/c_\mathrm{h}\right)\mathbf{C}^{-1} & \mathbf{C}\left(\boldsymbol{\alpha}_\mathrm{mm}/(c_\mathrm{h}Z_\mathrm{h})\right)\mathbf{C}^{-1}\end{pmatrix}.\end{aligned} \tag{3}$$

This equation consists of simple matrix multiplications, where $\mathbf{C}$ is a unitary matrix which transforms the polarizability tensors from the Cartesian to the spherical basis. With quantum-chemical methods, the dipolar polarizability tensors $\boldsymbol{\alpha}_{\nu\nu'}$ can be computed, which are complex $3 \times 3$ matrices. Such an *ab initio* quantum mechanical method is TD-DFT, for instance[2,4,5].

A molecular crystal consists of several stacked molecular two-dimensional lattices. The multi-scattering response of such a lattice is[3]

$$\boldsymbol{c}_{0,\mathrm{tot}} = \left(\mathbb{1} - \mathbf{T}\sum_{\boldsymbol{R}\neq 0}\mathbf{C}^{(3)}(-\boldsymbol{R})\mathrm{e}^{\mathrm{i}\boldsymbol{k}_\parallel\boldsymbol{R}}\right)^{-1}\mathbf{T}\boldsymbol{a}_0. \tag{4}$$

$\boldsymbol{R}$ is a point in the two-dimensional lattice, $\boldsymbol{k}_{\|}$ is the component of the originally illuminating plane wave parallel to the lattice, and $\mathbf{C}^{(3)}(-\boldsymbol{R})$ is a matrix consisting of translation coefficients for vector spherical waves. $\boldsymbol{a}_0$ consists of the expansion coefficients of the primary incident field and $\boldsymbol{c}_{0,\text{tot}}$ consists of the expansion coefficients of the total field scattered by an object at the origin of the lattice.

By solving Equation (4) and computing the respective Q-matrices defined in Equations (6)-(9) and (12a,b) in[3], the linear optical interaction between two-dimensional lattices with the same lattice vectors and isotropic slabs can be computed.

## II. DETAILS OF THE DENSITY FUNCTIONAL THEORY CALCULATIONS

In our novel multi-scale approach to study nonlinear optical materials and devices, we apply a bottom-up approach based on precise quantum chemistry calculations utilizing density functional theory (DFT) and its time-dependent linear response counterpart (TD-DFT). Upon converging the ground state electron density for the finite size molecular model of the crystalline Urea material, we proceed to calculate complex polarizability tensors (electric-electric, electric-magnetic and magnetic-magnetic) followed by the complex electric-electric first hyperpolarizabilities. For the latter calculations, we extended the existing implementation of the calculation of the real first hyperpolarizabilities in the development version of the TURBOMOLE electronic structure package[6] to complex frequencies. The combination of the efficient resolution-of-identity (RI) algorithm[7,8] combined with the multipole-accelerated resolution-of-identity (marij) algorithm[9] and the semi-numerical calculation of the exchange[10] contribution to the total electronic Hamiltonian allowed us to apply our methodology to large molecular models and large number of frequencies, previously inaccessible to us.

We start by defining the finite size molecular model of the Urea crystalline material which contains 2x2x2 unit cells obtained from the work of Guth *et al.*[11] Our molecular model consists of 16 Urea molecules and 128 atoms in total, depicted in Figure 2 of the manuscript. Urea crystallizes in a primitive tetragonal unit cell. The periodic cell of the finite size molecular model used in (TD-)DFT calculations thus has the following cell vector lengths: $a = b = 11.156$ Å and $c = 9.39$ Å.

For all calculations a hybrid B3LYP exchange-correlation functional[12,13] and def2-TZVP basis set was chosen[14,15]. The dynamic polarizabilities were calculated for the wavelength range 482 - 582 nm with the resolution of 1 nm and 964 - 1164 nm with the resolution of 2 nm. The damped

first hyperpolarizabilities were calculated for the wavelength range of ±100 nm around 1064 nm with the same resolution in that spectral range corresponding to 2 nm. In both cases a damping of 0.05 eV was applied to obtain the imaginary part of the (hyper)polarizabilities.

The complete set of quantum chemistry calculations based on TD-DFT method produced for this study is deposited in the NOMAD materials science database under the following DOI link: https://doi.org/10.17172/NOMAD/2023.08.31-1

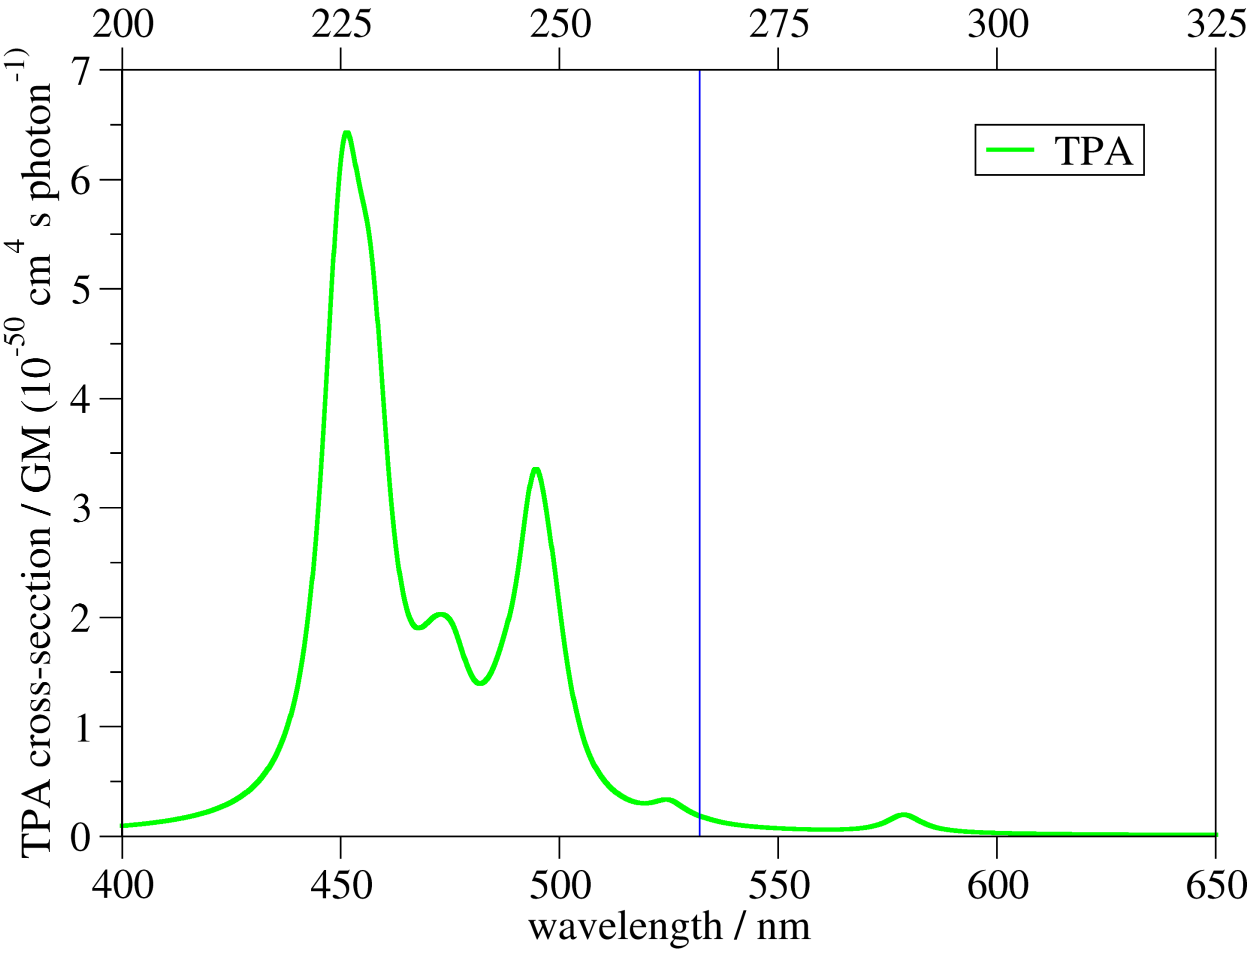


FIG. S1: Two-photon absorption (TPA) of the same Urea molecular model showing negligible TPA cross-sections around 532 nm (blue vertical line).

## REFERENCES


[1] P. Waterman, "Matrix formulation of electromagnetic scattering," *Proceedings of IEEE* **53**, 805–812 (1965).

[2] I. Fernandez-Corbaton, D. Beutel, C. Rockstuhl, A. Pausch, and W. Klopper, "Computation of electromagnetic properties of molecular ensembles," *ChemPhysChem* **21**, 878–887 (2020).

[3] D. Beutel, A. Groner, C. Rockstuhl, and I. Fernandez-Corbaton, "Efficient simulation of bi-periodic, layered structures based on the t-matrix method," Journal of the Optical Society of America B **38**, 1782–1791 (2021).

[4] B. Zerulla, M. Krstić, D. Beutel, C. Holzer, C. Wöll, C. Rockstuhl, and I. Fernandez-Corbaton, "A multi-scale approach for modeling the optical response of molecular materials inside cavities," *Advanced Materials* **34**, 2200350 (2022).

[5] B. Zerulla, C. Li, D. Beutel, S. Oßwald, C. Holzer, J. Bürck, S. Bräse, C. Wöll, I. Fernandez-Corbaton, L. Heinke, C. Rockstuhl, and M. Krstić, "Exploring functional photonic devices made from a chiral metal–organic framework material by a multiscale computational method," Advanced Functional Materials **n/a**, 2301093.

[6] "TURBOMOLE 7.7," (2022).

[7] K. Eichkorn, O. Treutler, H. Öhm, M. Häser, and R. Ahlrichs, "Auxiliary basis sets to approximate Coulomb potentials (Chem. Phys. Letters 240 (1995) 283-290)," Chemical Physics Letters **242**, 652–660 (1995).

[8] K. Eichkorn, F. Weigend, O. Treutler, and R. Ahlrichs, "Auxiliary basis sets for main row atoms and transition metals and their use to approximate Coulomb potentials," Theor Chem Acta **97**, 119–124 (1997).

[9] M. Sierka, A. Hogekamp, and R. Ahlrichs, "Fast evaluation of the Coulomb potential for electron densities using multipole accelerated resolution of identity approximation," The Journal of Chemical Physics **118**, 9136–9148 (2003).

[10] C. Holzer, "An improved seminumerical Coulomb and exchange algorithm for properties and excited states in modern density functional theory," The Journal of Chemical Physics **153**, 184115 (2020).

[11] H. Guth, G. Heger, S. Klein, W. Treutmann, and C. Scheringer, "Strukturverfeinerung von harnstoff mit neutronenbeugungsdaten bei 60, 123 und 293 K und x-n- und x-x(1s2)-synthesen bei etwa 100 K," Zeitschrift für Kristallographie - Crystalline Materials **153**, 237–254 (1980).

[12]A. D. Becke, "Density-functional thermochemistry. III. The role of exact exchange," The Journal of Chemical Physics **98**, 5648–5652 (1993).

[13]C. Lee, W. Yang, and R. G. Parr, "Development of the colle-salvetti correlation-energy formula into a functional of the electron density," Physical Review B **37**, 785–789 (1988).

[14]F. Weigend and R. Ahlrichs, "Balanced basis sets of split valence, triple zeta valence and quadruple zeta valence quality for H to Rn: Design and assessment of accuracy," Physical Chemistry Chemical Physics **7**, 3297–3305 (2005).

[15]F. Weigend, "Accurate Coulomb-fitting basis sets for H to Rn," Physical Chemistry Chemical Physics **8**, 1057–1065 (2006).
